# Supplementary material for: Multivariate conditional randomisation tests with unknown covariate parameters
Source: arXiv:2504.06685 source file (2026-11-27)
Supplement: Supplementary file 1 [file table-4-eta=0.1.tex]

\begin{tabular}{ll|cccccc}
\hline
& & \multicolumn{6}{c}{Method} \\ 
$q$ & $n$ & \nameVV & \nameDP & PRC & ERC & F-${\sum}$ & \multicolumn{1}{c}{F-max} \\ 
\hline
\hline 0.1 & 10  & \textbf{0.852 (.032)} & 0.352 (.042) & 0.289 (.040) & 0.367 (.043) & \textbf{0.852 (.032)} & 0.844 (.032) \\
 & 15  & 0.922 (.024) & 0.523 (.044) & 0.453 (.044) & 0.391 (.043) & 0.922 (.024) & \textbf{0.930 (.023)} \\
 & 30  & \textbf{0.977 (.013)} & 0.758 (.038) & 0.609 (.043) & 0.453 (.044) & 0.961 (.017) & \textbf{0.977 (.013)} \\
\hline 0.4 & 10  & 0.961 (.017) & 0.867 (.030) & 0.883 (.029) & 0.930 (.023) & \textbf{0.969 (.015)} & 0.961 (.017) \\
 & 15  & \textbf{0.992 (.008)} & 0.977 (.013) & 0.953 (.019) & 0.930 (.023) & \textbf{0.992 (.008)} & \textbf{0.992 (.008)} \\
 & 30  & 0.992 (.008) & \textbf{1.000 (.000)} & 0.977 (.013) & 0.945 (.020) & 0.992 (.008) & 0.992 (.008) \\
\hline 1 & 10  & 0.992 (.008) & 0.992 (.008) & \textbf{1.000 (.000)} & 0.992 (.008) & 0.992 (.008) & 0.992 (.008) \\
 & 15  & 0.992 (.008) & \textbf{1.000 (.000)} & \textbf{1.000 (.000)} & \textbf{1.000 (.000)} & \textbf{1.000 (.000)} & \textbf{1.000 (.000)} \\
 & 30  & \textbf{1.000 (.000)} & \textbf{1.000 (.000)} & \textbf{1.000 (.000)} & \textbf{1.000 (.000)} & \textbf{1.000 (.000)} & \textbf{1.000 (.000)} \\
\hline 
\end{tabular}
