# Supplementary material for: Multivariate conditional randomisation tests with unknown covariate parameters
Source: arXiv:2504.06685 source file (2026-11-27)
Supplement: Supplementary file 2 [file table-4-eta=0.15.tex]

\begin{tabular}{ll|cccccc}
\hline
& & \multicolumn{6}{c}{Method} \\ 
$q$ & $n$ & \nameVV & \nameDP & PRC & ERC & F-${\sum}$ & \multicolumn{1}{c}{F-max} \\ 
\hline
\hline 0.1 & 10  & 0.367 (.043) & 0.031 (.015) & 0.055 (.020) & 0.125 (.029) & \textbf{0.414 (.044)} & 0.305 (.041) \\
 & 15  & 0.570 (.044) & 0.195 (.035) & 0.164 (.033) & 0.148 (.032) & \textbf{0.586 (.044)} & 0.578 (.044) \\
 & 30  & 0.781 (.037) & 0.406 (.044) & 0.258 (.039) & 0.180 (.034) & 0.789 (.036) & \textbf{0.797 (.036)} \\
\hline 0.4 & 10  & 0.750 (.038) & 0.469 (.044) & 0.430 (.044) & 0.500 (.044) & \textbf{0.852 (.032)} & 0.680 (.041) \\
 & 15  & 0.930 (.023) & 0.758 (.038) & 0.805 (.035) & 0.695 (.041) & \textbf{0.984 (.011)} & 0.930 (.023) \\
 & 30  & \textbf{0.992 (.008)} & 0.969 (.015) & 0.953 (.019) & 0.883 (.029) & \textbf{0.992 (.008)} & \textbf{0.992 (.008)} \\
\hline 1 & 10  & 0.883 (.029) & 0.914 (.025) & \textbf{1.000 (.000)} & \textbf{1.000 (.000)} & 0.992 (.008) & 0.898 (.027) \\
 & 15  & 0.969 (.015) & 0.992 (.008) & \textbf{1.000 (.000)} & \textbf{1.000 (.000)} & \textbf{1.000 (.000)} & \textbf{1.000 (.000)} \\
 & 30  & \textbf{1.000 (.000)} & \textbf{1.000 (.000)} & \textbf{1.000 (.000)} & \textbf{1.000 (.000)} & \textbf{1.000 (.000)} & \textbf{1.000 (.000)} \\
\hline 
\end{tabular}
